# Supplementary material for: SoK: Kicking CAN Down the Road. Systematizing CAN Security Knowledge
Source: arXiv:2510.02960 source file (2026-09-25)
Supplement: Supplementary file 1 [file Appendix_CryptoIssues.tex]

%\subsection{Attack Defense Juxtaposition}\label{A:juxtaposition}


%To identify highly replicable attacks and attacks with defense gaps, we list all attacks and their replicability assessment and juxtapose them against possible defenses along with their effectiveness assessment against these attacks in Tbl. \ref{tbl:bigtable}. A \textit{gap} is a \textit{highly-replicable attack} (Sec. \ref{subsec:AttackAssessment}) for which there is no \textit{effective defense} (Sec. \ref{subsec:DefenseAssessment}). The left side lists attacks and their assessment. Possible defenses, per attack, and their assessment are on the right. Attacks appear once while defenses may appear more, with varying assessments, if they work for different attacks. Defense assessments apply to all applicable attacks on the left. Some attacks may have similar possible defenses. We cluster defenses that could work for any of them together. Dashed lines mean the defenses above the line apply to the attacks below the line, but the defenses below the line do not apply to the attacks above the line. Dotted lines signify the opposite. For example, \textit{\textit{bit-bang} IDS} works for \textit{frame hijacking}, but \textit{ID anonymization} does not work for \textit{unorthodox frames}. 


%We highlight highly-replicable attacks in light \textit{brown} and \textit{blue} for \textit{by-the-rulers} and \textit{bit-bangers}, and gaps in dark \textit{red} and \textit{blue}, respectively. As shown in the table, $8$ highly replicable attacks were identified to have defense gaps: \textit{1) Communication Surveillance,} since its only preventative solution is encryption and obfuscation but without full coverage due to the internal-attacker issue (\DCa). \textit{2) Fake Data Fabrication,} since Content inspection has coverage, system understanding, and modeling challenges (\DIb). \textit{3) Double Receive} is clustered in the table with other attacks (e.g., frame hijacking). Bit-banger IDS works well for the entire cluster except \textit{double receive} (hence the half coverage). Dynamic fragmentation and ECU guardians are the only possible preventions, but at a high infrastructure cost. \textit{4) Bus Access Denial and 5) Synchronization Disruption} have defense gaps only for \textit{bit-banger}s as layer-II node suspension (\DAd) works efficiently for \textit{by-the-ruler}s. While Dynamic fragmentation and ECU guardians provide prevention but at a high infrastructure cost. Finally, \textit{6) Error Injection, 7) State Manipulation, and 8) Reconaissance}are gaps only for \textit{bit-banger}s as ID and IFS anonymization are effective against the same attacks launched \textit{by-the-ruler}s.


% protocols could few papers adressed the issue of revocation

% \kha{move the whole thing to the gap?}

 % Some methods may \cite{pfeiffer2017implementing, lu2019leap} use a central server for key establishment.

% Being a broadcast-based bus complicates key management. Specifically, proposing to use group keys \cite{woo2014practical, pfeiffer2017implementing, lu2019leap} does not account for insider attackers (C: $\LEFTcircle$). Using separate keys for each transmitting-receiving pair was also proposed \cite{pfeiffer2017implementing, lu2019leap}. However, this presents a problem to multi-receiver messages (highly used in broadcast-based systems) as such messages will have to be encrypted and sent several times, once for each receiver (Busload: $\CIRCLE$). It also consumes the limited ECU storage in case of a bus with many ECUs since each ECU will have to keep track of many keys and counters (E: $\CIRCLE$). Finally, key exchange also presents a challenge. While some researchers presented innovative solutions that exploit the physical and datalink characteristics of the CAN bus to exchange secret keys \cite{mueller2015plug, jain2016physical, pfeiffer2017implementing}, most solutions assume the presence of preshared keys, which could be dangerous to combine with group key encryption as the compromise of one node jeopardizes the security of the entire group (C: $\LEFTcircle$). 




% Some techniques attempted to reduce the overhead and busload impact (E: $\LEFTcircle$; B: $\Circle$); by using non-encryption based obfuscation techniques such as Fisher–Yates shuffling \cite{fisher1957statistical, yeom2020methodology}. However, this does not work well for messages with messages carrying single-value signals (e.g., all 0s or 1s). S2-CAN \cite{pese2021s2} tried solving this problem using both insertion and shuffling. Nonetheless, both techniques are subject to the key management challenge. 
