# Supplementary material for: SoK: Kicking CAN Down the Road. Systematizing CAN Security Knowledge
Source: arXiv:2510.02960 source file (2026-09-25)
Supplement: Supplementary file 3 [file Appendix_IVBRevised.tex]

\clearpage

\begin{figure}[t]
  \centering
  \includegraphics{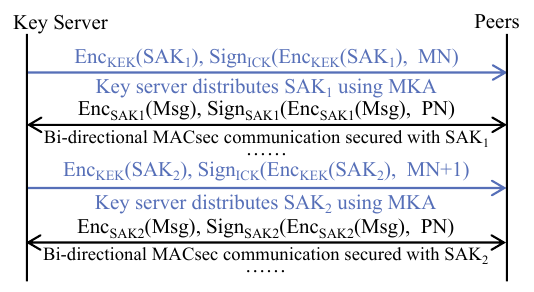}
  \caption{MACsec and MKA.}
  \label{fig:macsec}
\end{figure}

\section*{CANsec / MACsec Formal Verification}\label{inv:CANsec}


% \shortsectionEmph{MACsec Formal Verification:} \kha{appendix}MACsec \cite{MACsec} is an established link-layer cryptographic security add-on for Ethernet variants. It uses MACsec Key Agreement (MKA) \cite{mka} to distribute keys. While MKA allows different authentication types, current IV solutions are less flexible (e.g., AUTOSAR only supports PSK \cite{autosarmka}). Accordingly, we formally verify the de facto automotive MACsec with PSK. We report the results here and discuss the details in App. \ref{inv:CANsec}. As shown in Tbl. \ref{tbl:CANsec}, MACsec with PSK provides authenticity, freshness, and confidentiality only against external but not \textit{internal attackers} ($\mathcal{DR}1$) and thus does not close any defense gaps. 

% \shortsectionEmph{MACsec+:} \kha{appendix or remove. Maybe also put it as a takeaway: Revocation may close this gap} We propose and verify that a hypothetical improvement which integrates MACsec with a generic dynamic revocation protocol closes the gap. Similar to CANsec+, this requires changing the current automotive PSK setup.

We formally verify CANsec and MACsec, the standardized link-layer cryptographic add-on of CAN XL and 10BASE-T1S, to understand if they address the \textit{internal attacker} issue ($\mathcal{DR}$1). We first introduce the CANsec and MACsec protocols (Sec. \SecA), define the security properties to be verified (Sec. \SecB), and verify CANsec/MACsec as they currently stand, showing they cannot close the \textit{internal attacker} gap (Sec. \SecC). Finally, to investigate how to close this gap, we test the hypothesis that if a protocol to dynamically revoke compromised ECUs exists, this gap can be addressed (Sec. \SecD). 


\subsection{Protocols Overview}\label{cansec:overview}

\shortsectionBf{MACsec.} MACsec is a link-layer security add-on standardized by IEEE and is compatible with all Ethernet variants \cite{MACsec}. It provides message authenticity, freshness, and confidentiality. It can be implemented in hardware to operate at line speed. Nodes taking part in MACsec communication form a secure Connectivity Association (CA) and share a long-term Connectivity Association Key (CAK). Using MACsec Key Agreement (MKA) \cite{mka}, nodes authenticate each other, distribute short-term Secure Association Keys (SAK), and use them to secure communication as described below:\looseness-1 


% It uses MACsec Key Agreement (MKA) \cite{mka} to distribute keys. While MKA allows different authentication types, current IV solutions are less flexible (e.g., AUTOSAR only supports PSK \cite{autosarmka}). Accordingly, we formally verify the de facto automotive MACsec with PSK.

\shortsectionEmph{MACsec Key Agreement:} MKA supports many configurations and optional features, such as different authentication types, key server election, etc. However, current in-vehicle solutions are less flexible (automotive MKA  \cite{automotive_mka} and AUTOSAR \cite{autosarmka} only support pre-shared keys). Accordingly, the de facto automotive setup uses pre-shared CAK (PSK) with a fixed key server performing the basic function of distributing SAKs to peers. Fig. \ref{fig:macsec} shows a simplified illustration. A key server periodically generates new SAKs and distributes them using MKA messages containing the encrypted SAKs using a Key Encryption Key (KEK), an incrementing message number (MN), and an Integrity Check Value (ICV) calculated for the message using an ICV Key (ICK). Both KEK and ICK are derived from the CAK. Peers verify the ICV and MN, and install the new SAK. Subsequent MACsec messages contain an ICV generated for its content (optionally encrypted with SAK) and an incrementing Packet Number (PN) using the SAK to provide authenticity, freshness, and optional confidentiality. 


  % Keys are agreed on using CKA \cite{CKA} and pre-shared keys (PSKs). We obtained a working draft by reaching out to the CAN in Automation (CiA) organization \kha{fix reference}. Here, we report the outcome of our verification. The details are in App. \ref{inv:CANsec}. As shown in Tbl. \ref{tbl:CANsec}, as the current CKA setup stands, CANsec provides authenticity, freshness, and confidentiality only against external attackers but not \textit{internal attackers} ($\mathcal{DR}1$) and hence does not close any open defense gaps. 



\shortsectionBf{CANsec.} Modeled after MACsec, CANsec is an in-development link-layer security add-on for CAN XL \cite{CANsec}. We obtained a draft by contacting the CAN in Automation (CiA) organization. In the current proposal, CANsec uses the same concepts of CA, CAK, and ICV generation using SAK and incrementing PN. Unlike MACsec, some message fields (e.g., priority ID) are excluded from ICV protection. Mechanisms for CA establishment and member authentication is in early development. Pre-shared CAK is likely since AUTOSAR suggests it for MACsec, with voices proposing keeping it authentication-agnostic for flexible integration with other protocols. CANsec uses CANsec Key Agreement (CKA) to distribute SAKs. CKA is in early development with two approaches being debated: 1) Modeled after MKA, and 2) In-line Key Agreement (IKA) \cite{zeh2025secure} as explained below:

\shortsectionEmph{In-line Key Agreement:} Fig. \ref{fig:cansec} is a simplified illustration of IKA. SAKs are derived using the CAK, an incrementing Key Number (KN), and a Key Derivation Function (KDF). A transmitter includes the current KN, an incrementing PN, an optionally encrypted payload, and an ICV calculated using the current SAK in a regular CANsec message. On receiving a new KN, a receiver derives a new SAK using the CAK, KN, and KDF, and uses it for subsequent communication if the message's ICV is verified using the new SAK.

\subsection{Security Properties}\label{cansec:properties}

We assume the attacker is a \textit{by-the-ruler} following the Dolev-Yao model with two variations: an \textit{external (E)} attacker who is not a member of a CA, and an \textit{internal (I)} attacker who is a compromised member-ECU of the CA and has access to the ECU's CAK and SAK. We verify the following security properties against both \textit{E} and \textit{I} attackers:

\vspace{7pt}
%\setlist[itemize]{leftmargin=*}
\noindent\fbox{\begin{minipage}{\columnwidth-2\fboxsep-2\fboxrule}
\footnotesize
\centering
\begin{itemize}[itemsep=3pt]
    \itemindent=-17pt
    \item[]$\mathcal{P}_{a}$$\mathtt{: Attacker}$ $\mathtt{cannot}$ $\mathtt{spoof}$ $\mathtt{CA}$ $\mathtt{messages}$ $\mathtt{or}$ $\mathtt{distributed}$ $\mathtt{SAKs}$
    \item[]$\mathcal{P}_{f}$$\mathtt{: Attacker}$ $\mathtt{cannot}$ $\mathtt{replay}$ $\mathtt{CA}$ $\mathtt{messages}$ $\mathtt{or}$ $\mathtt{distributed}$ $\mathtt{SAKs}$
    \item[]$\mathcal{P}_{c}$$\mathtt{: Attacker}$ $\mathtt{cannot}$ $\mathtt{surveil}$ $\mathtt{encrypted}$ $\mathtt{CA}$ $\mathtt{messages}$ $\mathtt{or}$ $\mathtt{obtain}$ $\mathtt{distributed}$ $\mathtt{SAKs}$
\end{itemize}
\end{minipage}}

\begin{figure}[t]
  \centering
  \includegraphics{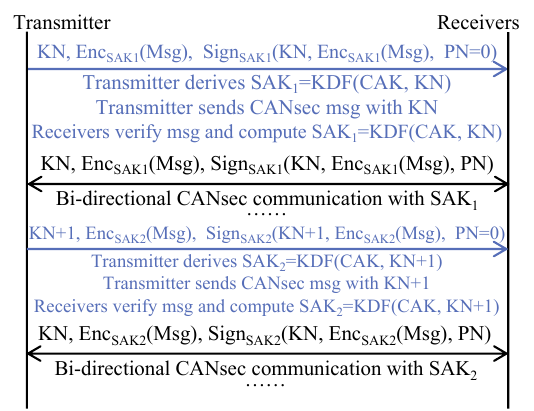}
  \caption{CANsec and IKA.}
  \label{fig:cansec}
\end{figure}

%\shortsectionBf{Security Properties.} We verify these security properties:
%\vspace{7pt}
%\setlist[itemize]{leftmargin=*}
%\noindent\fbox{\begin{minipage}{23.5em}
%\small
%\centering
%\begin{itemize}[itemsep=3pt]
%    \itemindent=-17pt
%    \item[]$\mathcal{P}_{a}$$\mathtt{: Attacker}$ $\mathtt{cannot}$ $\mathtt{spoof}$ $\mathtt{CA}$ $\mathtt{messages}$
%    \item[]$\mathcal{P}_{f}$$\mathtt{: Attacker}$ $\mathtt{cannot}$ $\mathtt{replay}$ $\mathtt{CA}$ $\mathtt{messages}$
%    \item[]$\mathcal{P}_{c}$$\mathtt{: Attacker}$ $\mathtt{cannot}$ $\mathtt{surveil}$ $\mathtt{encrypted}$ $\mathtt{CA}$ $\mathtt{messages}$
%    \item[]$\mathcal{P}_{r}$$\mathtt{: Revoking}$ $\mathtt{CA}$ $\mathtt{members}$ $\mathtt{dynamically}$ $\mathtt{is}$ $\mathtt{possible}$
%\end{itemize}
%\end{minipage}}

%\vspace{7pt}

%\shortsectionBf{Model Design.}  We formally model the protocols using ProVerif \footnote{Code link: \url{https://anonymous.4open.science/r/IVB_verification-0DF8}} \cite{blanchet2016modeling}. We consider the following scenarios: %We use two processes to model a transmitter and receiver. The transmitter derives and distributes SAKs, and continuously transmits messages, encrypted and signed with the SAK and an incrementing counter. A receiver verifies and installs SAKs, authenticates the received messages, checks the freshness of the counters, and finally decrypts to obtain the plaintext message.  

\subsection{CANsec/MACsec Verification}\label{cansec:modeling}

To verify the properties in Sec. \SecB, we model MACsec/MKA and CANsec/CKA using ProVerif \cite{blanchet2016modeling}.

\shortsectionEmph{MACsec:} We model MACsec with statically configured CA as it currently stands based on relevant automotive standards \cite{automotive_mka,autosarmka}. We use two processes to model a transmitter and receiver sharing an SAK. The transmitter continuously transmits messages containing a payload. The transmitter encrypts the payload with the SAK, and appends an ICV calculated using the SAK, an incrementing PN, and payload. A receiver verifies the ICV, checks the freshness of the PN, and finally decrypts to obtain the plaintext payload. We verify $\mathcal{P}_{a}$, $\mathcal{P}_{f}$, and $\mathcal{P}_{c}$ on the encrypted and authenticated payload for both \textit{E} attackers not knowing the SAK and \textit{I} attackers knowing the SAK.

\shortsectionEmph{MKA:} We model MKA with a static key server based on the automotive MKA standard \cite{automotive_mka}. Two processes model a key server and a peer sharing a CAK. The key server continuously generates new SAKs, encrypts them with the KEK, and distributes SAKs in MKA messages signed with the ICK and an incrementing MN. The peer verifies the ICV, checks the MN's freshness, then decrypts and installs the new SAK. We verify $\mathcal{P}_{a}$, $\mathcal{P}_{f}$, and $\mathcal{P}_{c}$ on the distributed SAK for both \textit{E} attackers not knowing the CAK and \textit{I} attackers knowing the CAK.\looseness-1

\shortsectionEmph{CANsec:} We assume CA membership cannot be dynamically modified, as the current CANsec proposal does not outline a concrete mechanism supporting this \cite{CANsec}. Similar to MACsec, we use two processes to model a transmitter and receiver sharing an SAK and exchanging messages. Unlike MACsec, messages contain a priority ID and payload, and only the payload is encrypted and authenticated with the SAK. We verify $\mathcal{P}_{a}$, $\mathcal{P}_{f}$, and $\mathcal{P}_{c}$ on the encrypted and authenticated payload for both \textit{E} attackers not knowing the SAK and \textit{I} attackers knowing the SAK.\looseness-1

\shortsectionEmph{CKA:} Assuming PSKs, we model both two potential approaches of CKA: 1) MKA-like: we use the same model for MKA. 2) IKA: we have a key distribution process and an installation process share a CAK. The distribution process continuously increments a KN, derives new SAKs using the KN and CAK, and transmits messages authenticated and encrypted using the CAK. The installation process detects new KN, derives the new SAK, and installs it if the message is successfully verified using the new SAK. We verify $\mathcal{P}_{a}$, $\mathcal{P}_{f}$, and $\mathcal{P}_{c}$ on the distributed SAK for both \textit{E} attackers not knowing the CAK and \textit{I} attackers knowing the CAK.

\begin{tcolorbox}[
  colback=gray!15,
  colframe=gray!60,
  fonttitle=\bfseries,
    boxsep=0pt,
  left=2pt,
  right=2pt,
  top=2pt,
  bottom=2pt,
  before skip=4pt,
  after skip=4pt,
]
\shortsectionBf{CANsec/MACsec Verification Results} 

As shown in Tbl. \ref{tbl:CANsec}, as they currently stand, CANsec and MACsec provide authenticity, freshness, and confidentiality only against external attackers but unfortunately not \textit{internal attackers} and hence cannot close any open defense gaps\footnote{Conclusions for CANsec are based on its current proposal assuming PSKs. They may differ for the eventual standardized design.}.
\end{tcolorbox}


% \shortsectionEmph{CANsec+:}  \kha{appendix or remove} Fortunately, CANsec and CKA are still under development and could be improved to close the gap. We propose and verify that a hypothetical improved protocol, which integrates CANsec with a generic dynamic revocation protocol and does not rely on pre-shared keys, closes this gap.\looseness-1

\input{Tables/CANsec3}
\subsection{Impacts of Revocation}\label{cansec:revocation}

As we have shown, CANsec and MACsec in their current versions do not close the \textit{internal attacker} issue underlying many gaps. Fortunately, CANsec and CKA are still under development and could be improved to close the gap. We hypothesize that a dynamic near-immediate revocation protocol can close this gap. In this section, we test this hypothesis by assuming such a protocol exists and verify its impacts if integrated with CANsec/MACsec. Note that our goal is not to propose a concrete revocation protocol but rather to highlight the benefits of researching this direction.

\shortsectionBf{Assumptions on the Revocation Protocol.} We assume the revocation protocol meets two requirements: 1) It is immediate, starts once the compromised CA member is identified, and completes before any new CANsec or MACsec messages are exchanged; 2) It removes the compromised CA member from the CA and securely distributes new SAKs to remaining members. Subsequent communication only uses new SAKs, not SAKs previously compromised by the attacker. The details of such a revocation protocol are outside the scope of this study.\looseness-1

\shortsectionBf{Modeling the Impacts of Revocation.} We extend our CANsec/MACsec models with a new phase, where the transmitting and receiving processes use a new SAK not known by the attacker. This models the outcome of a revocation protocol satisfying the assumption described before: the attacker node is removed from the CA, and the remaining CA members communicate using securely distributed new SAKs. We verify $\mathcal{P}_{a}$, $\mathcal{P}_{f}$, and $\mathcal{P}_{c}$ on the encrypted and authenticated message payload for both \textit{E} attackers not knowing the SAK and \textit{I} attackers knowing only the previous compromised SAK. 

\begin{tcolorbox}[
  colback=gray!15,
  colframe=gray!60,
  fonttitle=\bfseries,
    boxsep=0pt,
  left=2pt,
  right=2pt,
  top=2pt,
  bottom=2pt,
  before skip=4pt,
  after skip=4pt,
]
\shortsectionBf{Benefits of Revocation} 

Assuming a dynamic near-immediate revocation protocol exists and is integrated with CANsec/MACsec, authenticity, freshness, and confidentiality can be provided against both external and internal attackers. This highlights that fast revocation can close the \textit{internal attacker} gap and is a worthwhile research direction.
\end{tcolorbox}

%\shortsectionIt{1) Static CANsec/MACsec:} Based on relevant automotive standards \cite{CANsec,automotive_mka,autosarmka} which do not support dynamic modification of CA membership,  we model CANsec/MACsec as they currently stand. We use two processes to model a transmitter and receiver sharing an SAK. The transmitter continuously transmits messages encrypted with the SAK, which contain an incrementing PN and ICV calculated using the SAK. A receiver verifies the ICV, checks the freshness of the PN, and finally decrypts to obtain the plaintext message. We verify $\mathcal{P}_{a}$, $\mathcal{P}_{f}$, and $\mathcal{P}_{c}$ for both \textit{E} attackers not knowing the SAK and \textit{I} attackers knowing the SAK. %Verification challenges arise because CANsec/MACsec keeps track of global states (e.g., the most recent PN) and Proverif fails to prove properties on such protocols due to its internal abstractions. We apply the transformations proposed by \cite{cheval2018little} to yield successful proofs. \kha{Your insistance on saying "we assume PSK" allover makes you come across insecure and begging for a question from a reviewer. Also, I am not sure why we are combinging CANsecn and MACsec rewrite} \kha{This is so vague. How did you do that? What challenges, etc}

%\shortsectionIt{2) CANsec+/MACsec+:} We verify a hypothetically improved protocol which integrates CANsec/MACsec with a generic dynamic revocation mechanism to revoke CA members upon their compromise. We assume the revocation mechanism meets the following requirements: 1) The revocation protocol is immediate, starts once the compromised CA member is identified, and completes before any new CANsec/MACsec messages are exchanged; 2) The protocol securely distributes new SAKs to remaining members, and subsequent communication does not use compromised SAKs. The details of this revocation mechanism are outside the scope of this study as any protocol meeting these requirements. We extend our static CANsec/MACsec models with a new phase, where the transmitting and receiving processes use a new SAK not known by the attacker, to model the effect of revocation. We verify $\mathcal{P}_{a}$, $\mathcal{P}_{f}$, and $\mathcal{P}_{c}$ for both \textit{E} attackers not knowing the SAK and \textit{I} attackers knowing only the previous compromised SAK.

%\shortsectionIt{3) CKA/MKA Revocation:} We model the current state of automotive CKA/MKA and verify if they meet the requirements on revocation protocols for CANsec+/MACsec+ ($\mathcal{P}_{r}$). We create separate models for MKA and IKA. A key distribution process continuously generates and distributes new SAKs following the steps in Fig. \ref{fig:macsec} and \ref{fig:cansec}. A key installation process verifies the received message and installs the new SAK. We verify if they support distributing SAKs securely when an \textit{I} attacker having the pre-shared CAK is present by checking if the attacker can obtain, spoof, or replay exchanges SAKs.

%\input{Tables/CANsec3}

%\shortsectionBf{Results.} As shown in Tbl. \ref{tbl:CANsec}, as they currently stand, CANsec and MACsec provide authenticity, freshness, and confidentiality only against external attackers but unfortunately not \textit{internal attackers} ($\mathcal{DR}1$) and hence do not close any open defense gaps. Luckily, our verification shows that integrating them with a fast revocation mechanism extends these security properties to \textit{internal attackers} and thus closes the gap. However, the current CKA proposal and the de facto automotive MKA setup do not support revocation as the security of distributed SAKs relies on the pre-shared CAK, which is known by an internal attacker. This allows an internal attacker to freely tamper with the SAK distribution, including obtaining, spoofing, and replaying exchanged SAKs. Thus, closing the \textit{internal attackers} gap requires a different mechanism from PSK. Fortunately, these protocols are still under development and could update their design to integrate such use cases.



% However, if the protocol could be extended to allow for dynamic and fast revocation of compromised nodes, it could provide the same properties against internal attackers as well. Unfortunately, revocation is impossible with PSKs for both possible approaches of CKA ($\mathcal{P}4$). Fortunately, CKA is still under development with some voices proposing to keep it authentication agnostic to allow it to be integrated with various protocols. 


% In conclusion, as it stands, CANsec alone still suffers from the \textit{internal attacker issue} discussed in $\mathcal{DR}1$ and hence does not close any open defense gaps. However, it lays the ground work for smart solutions (e.g., fast revocation) that could extend it to close open gaps.


% room for authentication to be agnostic


% CANsec statically cannot 
% However, dynamically, it can
% Unfortuantely, the current CKA proposal cannot
% Fortunately they are still under dev and some propose to leave room for authentication to be agnostic
% conclusion, it does not close gaps but lays  the groud work for closing if smart solutions pick up were they leave off
% likely to improve performance, provide fertile ground for development and could be extended to cover gaos but as it stands it still suffers from the same internal attacker problem

% . Based on $\mathcal{T}3$, we formally verify whether CANsec, could fill any security gaps or provide an efficient defense against any highly-replicable attacks. \kha{make convincing}
% Having identified the root causes behind the highly-replicable attacks and gaps. We try to answer whether future CAN alternatives are more secure by vetting them to see whether they share any common root-causes. We consult the standards of two CAN evolutions: CANFD and CANXL, and Automotive Ethernet 10BASE-T1S, an ethernet variant that aims to replace CAN. We discuss why we choose these three standards in App. \ref{}. 


% \kha{Here. same criteria for attacks + no rule violation. Finish this section then decide on the RC table and the takeway intro}
 % We base our selection of IVBs on two assumptions: \textit{wiring costs}, and \textit{convenience}. \kha{zonal, speed, etc?} The wiring harness is one of the most expensive parts of the vehicle \cite{Wiring2}, weighing $50-70kg$, it is currently the third heaviest part after the engine and chassis \cite{Wiring}. This limits our search two buses with at most a twisted pair of wires. Convenience suggests that manufacturers, already used to CAN, will not want to move away to a different protocol and will prefer another CAN variant. However, it may suggest as well that they choose another standard everyone is used to: Ethernet. As such, we believe CANFD, CANXL, or Automotive 10BASE-T1S are the most likely IVBs to replace CAN 2.0.

% % Despite several point-to-point and switched communication technologies finding their way onto automotive platforms, we believe that the wiring costs will put a limit on their prevalence. The wiring harness is one of the most expensive parts of the vehicle \cite{Wiring2}. Weighing $50-70kg$, and is currently the third heaviest part of the vehicle after the engine and the chassis \cite{Wiring}. As such, we expect that the bulk of in-vehicle communication will remain bus-based, and that point-to-point and switched technologies will coexist with buses and remain confined to the segments where there usage is necessary. Three bus technologies standout as future evolutions/replacements for CAN: CANFD, CANXL, and Automotive 10BASE-T1S Ethernet. We expect CANFD to only be transitory, while the real long-term evolution will be either CANXL, or 10BASE-T1S \cite{bosch2012can, CANXL, AEth10B}. Below, we review the standards of these three technologies and compare their security posture to CAN's using the identified high-replicability and defense gap root-causes from Sec. \ref{subsec:RC} and Sec. \ref{subsec:DRC}. \kha{Cost: Wiring and phy + Convenience: Established Ethernet and CAN, zonal architecture}
% % \input{Tables/CANAlts}
% (e.g., SerDes \cite{MIPI, ASA}) and switched (e.g., \cite{AEth100, AEth1000})
